# Supplementary material for: How Gamification Affects Physical Activity: Large-scale Analysis of Walking Challenges in a Mobile Application
Source: arXiv:1702.07437 source file (2017-02-24)
Supplement: Supplementary file 1 [file 080appendix.tex]

% !TEX root = paper-competition.tex

\newpage
\pagebreak

\begin{figure}[h!]
\centering
  \centering
  \includegraphics[width=0.5\columnwidth]{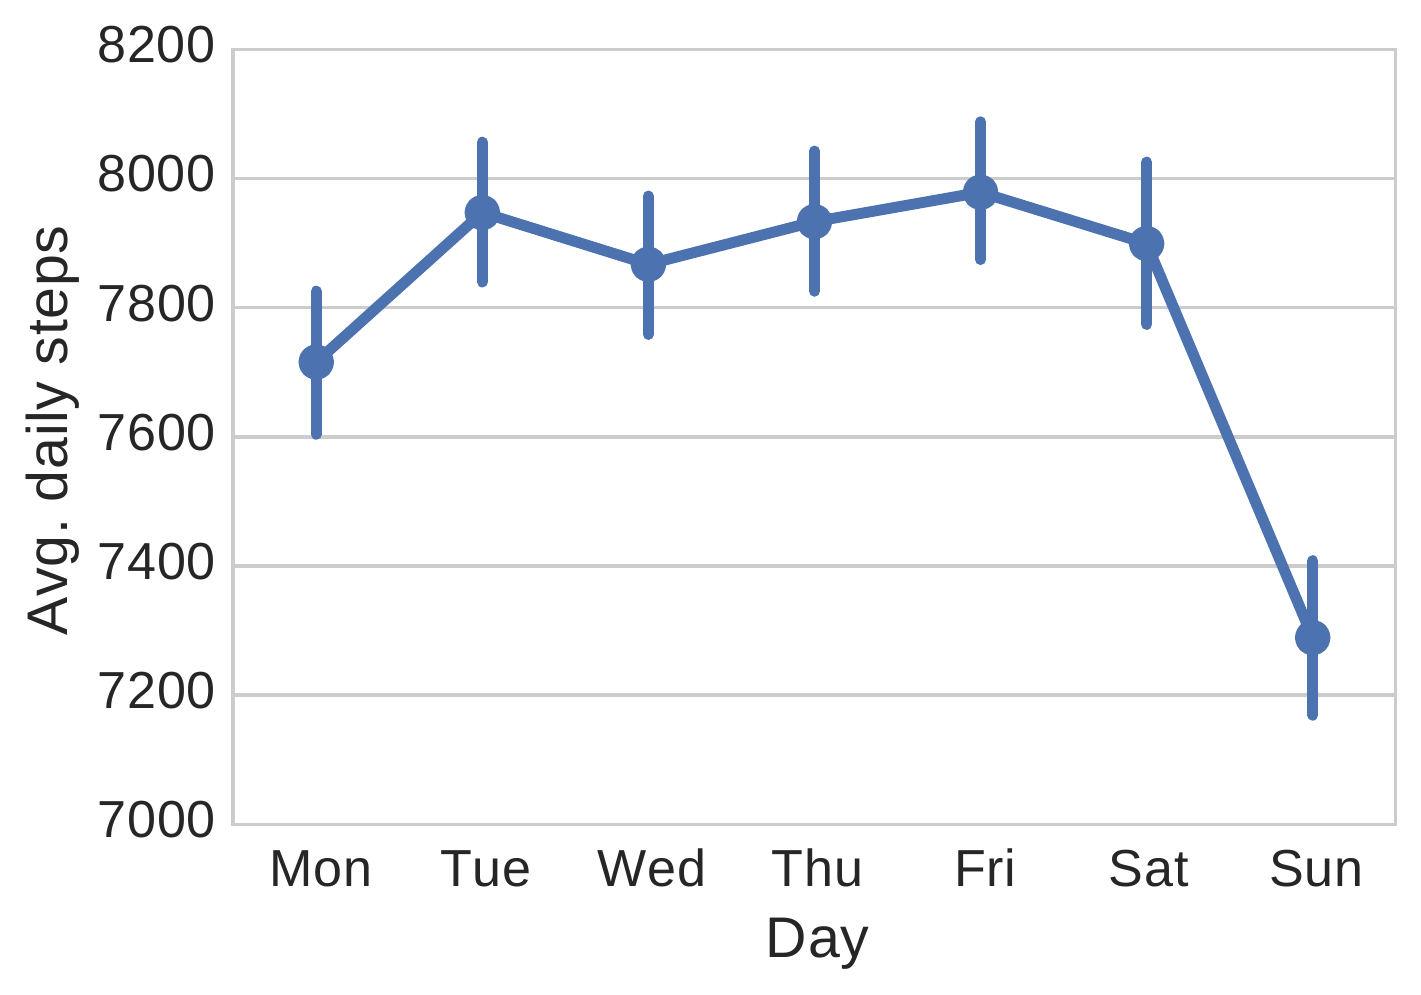}
  \captionof{figure}{\jure{This plot is not bad. We could maybe add it next to Figure 1} Average number of steps taken by users over different days of the week}
  %\label{fig:WWW-stepsperday}
\end{figure}

\begin{figure}[h!]
\centering
  \centering
  \includegraphics[width=0.5\columnwidth]{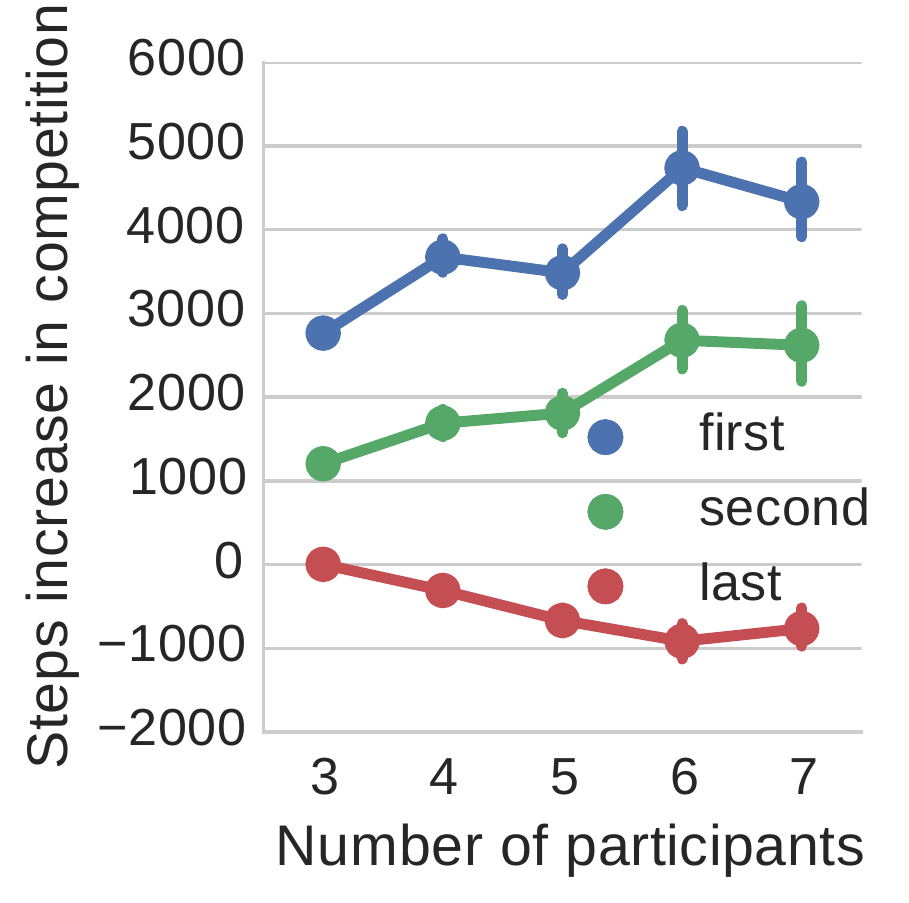}
  \captionof{figure}{Average number of steps taken by users specified by number of participants in the competition}
  %\label{fig:WWW_steps_per_counts}
\end{figure}

\begin{figure}[h!]
\centering
%\begin{minipage}{.47\columnwidth}
  \centering
  \includegraphics[width=0.5\columnwidth]{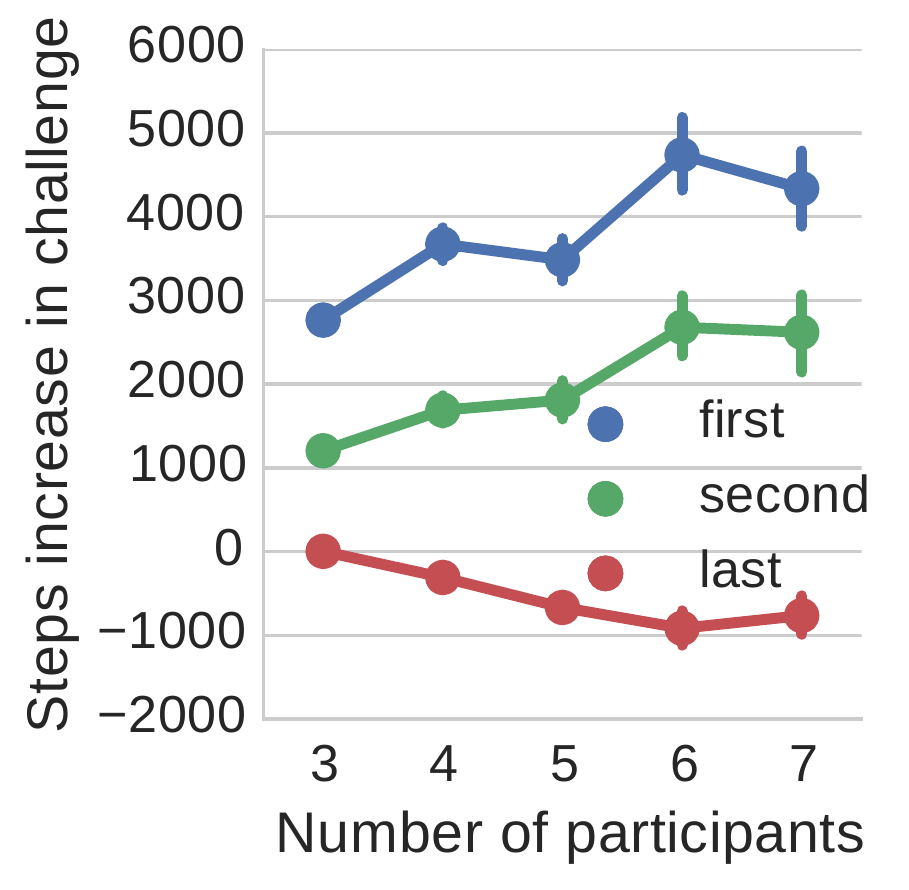}
  \captionof{figure}{Average increase in steps compared to previous outside competition activity specified by number of participants in the competition}
%\end{minipage}%
  %\label{fig:WWW_delta_steps_per_counts}
\end{figure}

\begin{figure}[h!]
\centering
%\begin{minipage}{.47\columnwidth}
  \centering
  \includegraphics[width=0.5\columnwidth]{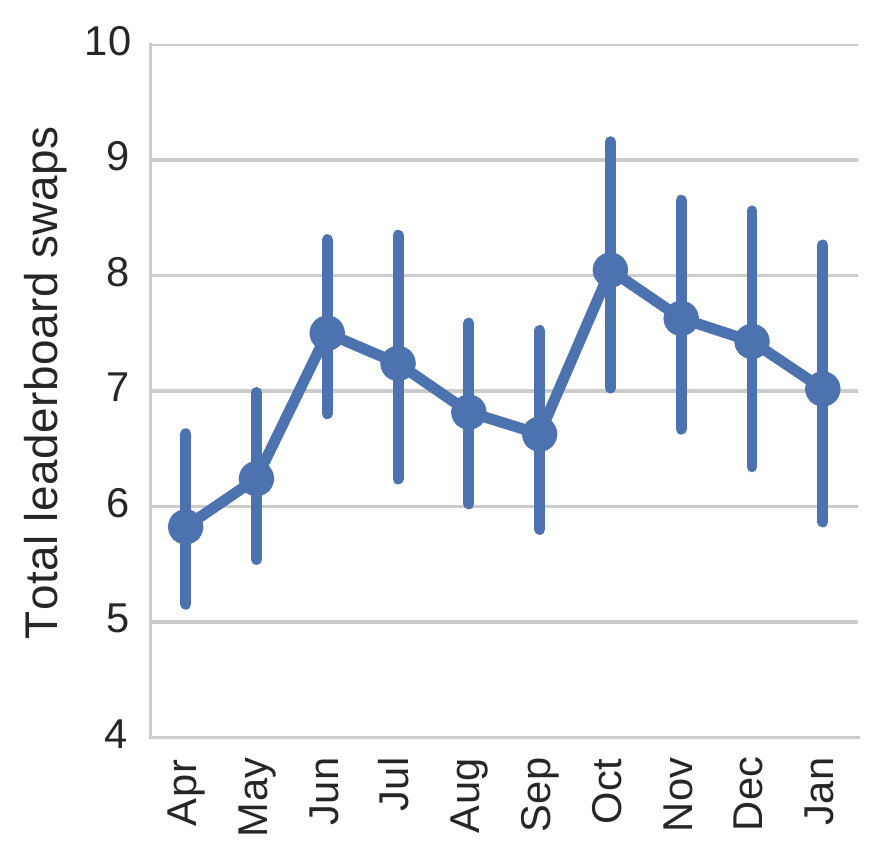}
  \captionof{figure}{Average number of swaps in the leaderboard for 7 day competitions with more than 2 participants}
%\end{minipage}%
  %\label{fig:WWW-leaderboard_changes_per_month_7participants}
\end{figure}

\begin{figure}[h!]
\centering
%\begin{minipage}{.47\columnwidth}
  \centering
  \includegraphics[width=0.5\columnwidth]{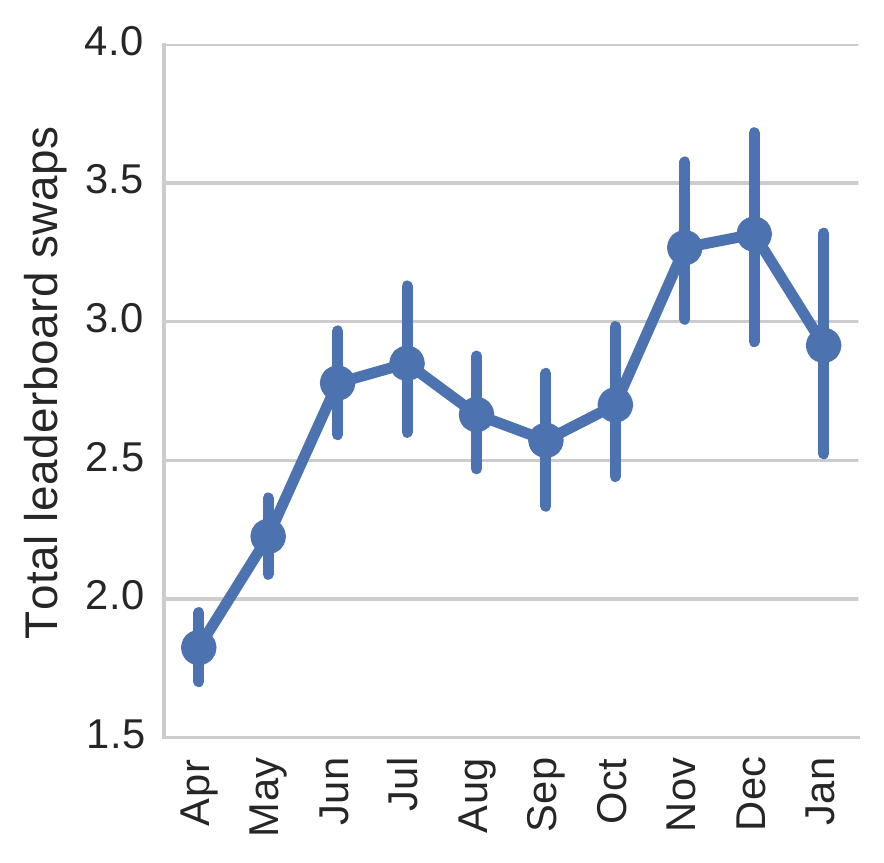}
  \captionof{figure}{Average number of swaps in the leaderboard for longer than 1 day competitions with more than 1 participants}
%\end{minipage}%
  %\label{fig:WWW_leaderboard_changes_per_month_7participants_longerthanone_morethanoneparticipants}
\end{figure}

\begin{figure}[h!]
\centering
%\begin{minipage}{.47\columnwidth}
  \centering
  \includegraphics[width=0.5\columnwidth]{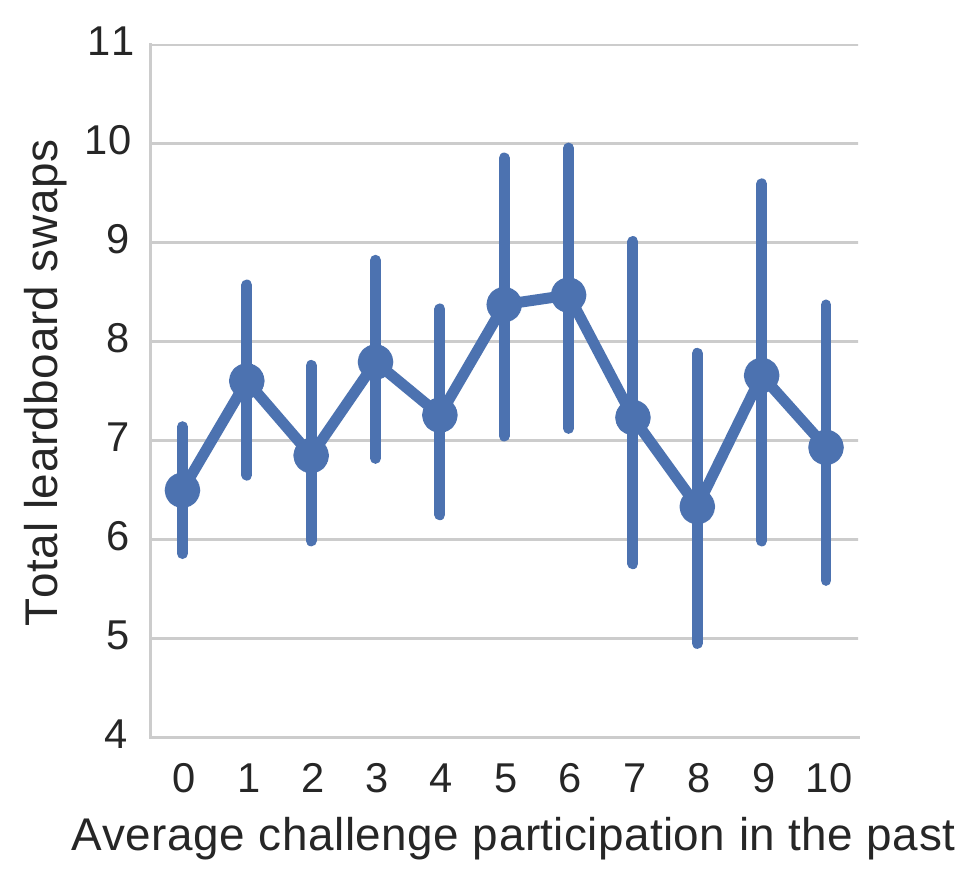}
  \captionof{figure}{Average number of swaps in the leaderboard for 7 day competitions with more than 2 participants}
%\end{minipage}%
  %\label{fig:WWW_leaderboard_changes_per_participation}
\end{figure}

\begin{figure}[h!]
\centering
%\begin{minipage}{.47\columnwidth}
  \centering
  \includegraphics[width=0.5\columnwidth]{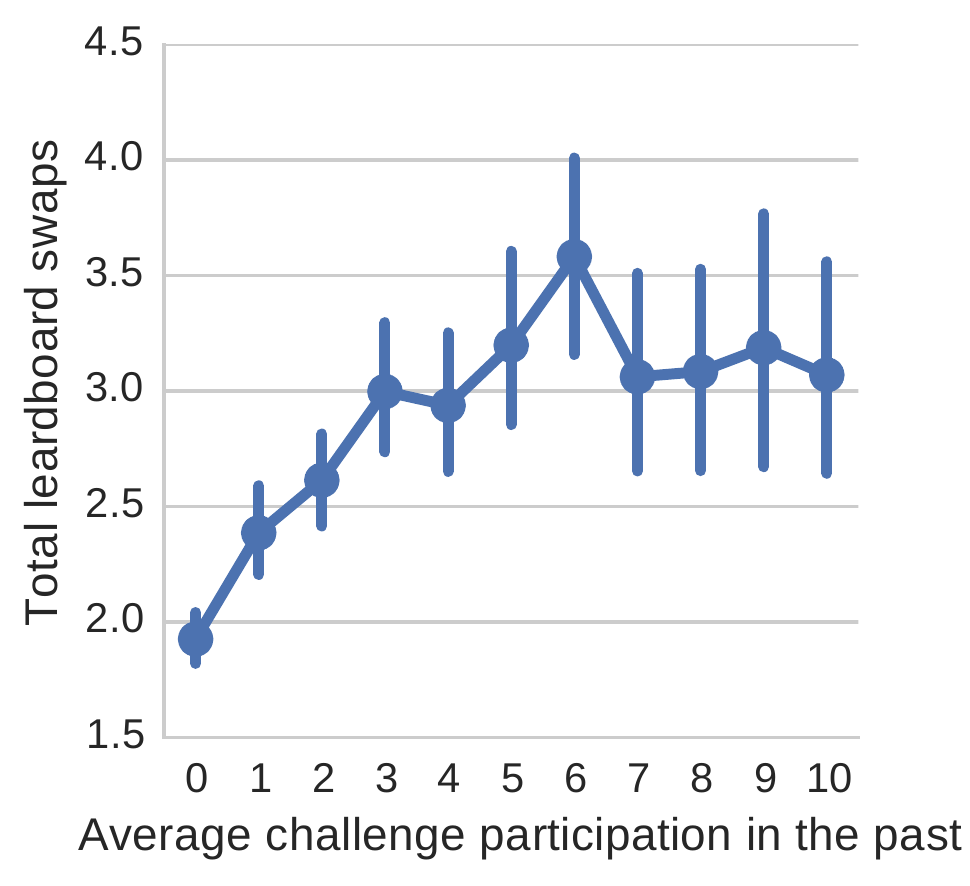}
  \captionof{figure}{Average number of swaps in the leaderboard for longer than 1 day competitions with more than 1 participants}
%\end{minipage}%
  %\label{fig:WWW_leaderboard_changes_per_participation_longerthanone_morethanoneparticipants}
\end{figure}

\begin{figure}[h!]
\centering
%\begin{minipage}{.47\columnwidth}
  \centering
  \includegraphics[width=0.5\columnwidth]{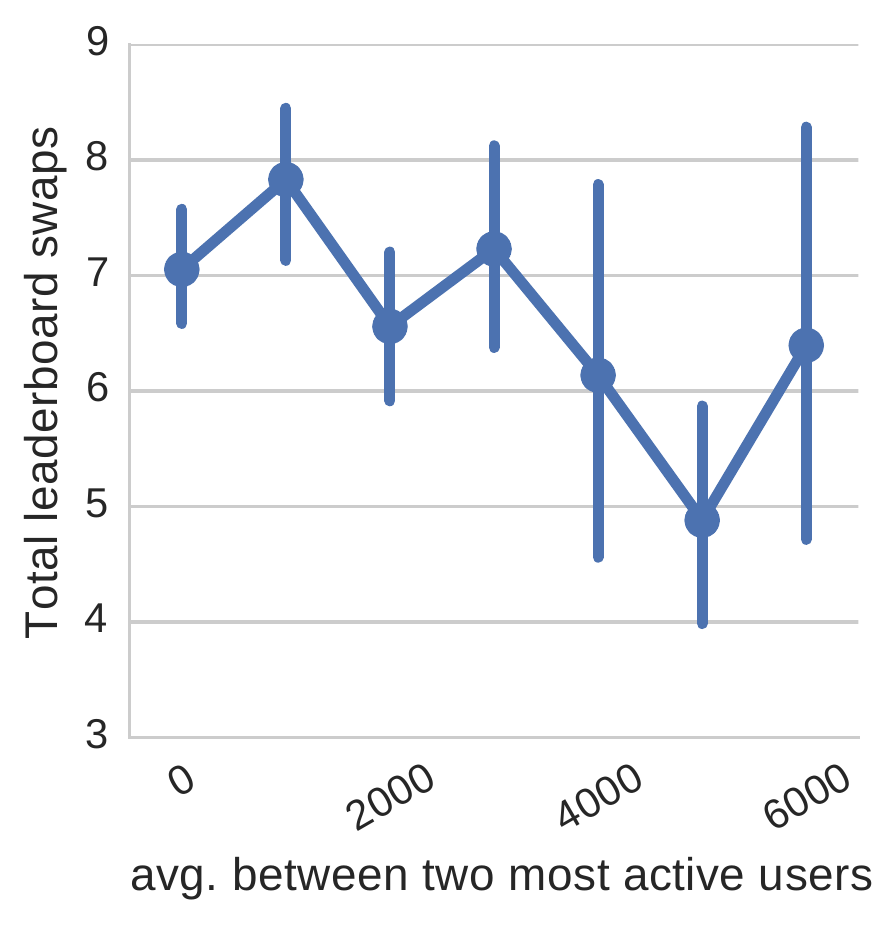}
  \captionof{figure}{Average number of swaps in the leaderboard for 7 day competitions with more than 2 participants based on the }
%\end{minipage}%
  %\label{fig:WWW_leaderboard_changes_per_difference}
\end{figure}

\begin{figure}[h!]
\centering
%\begin{minipage}{.47\columnwidth}
  \centering
  \includegraphics[width=0.5\columnwidth]{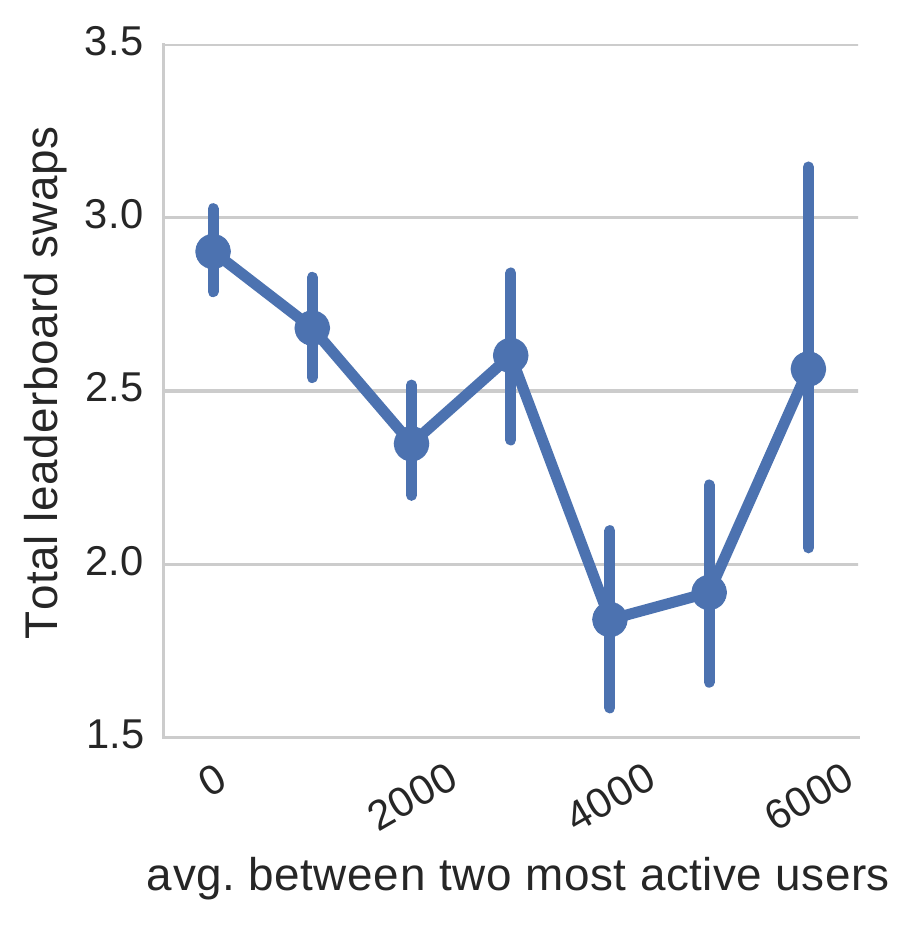}
  \captionof{figure}{Longer than 1 day competitions with more than 1 participants}
%\end{minipage}%
  %\label{fig:WWW_leaderboard_changes_per_difference_longerthanone_morethanoneparticipants}
\end{figure}

\begin{figure}[ht]
  \centering
  \includegraphics[width=0.5\columnwidth]{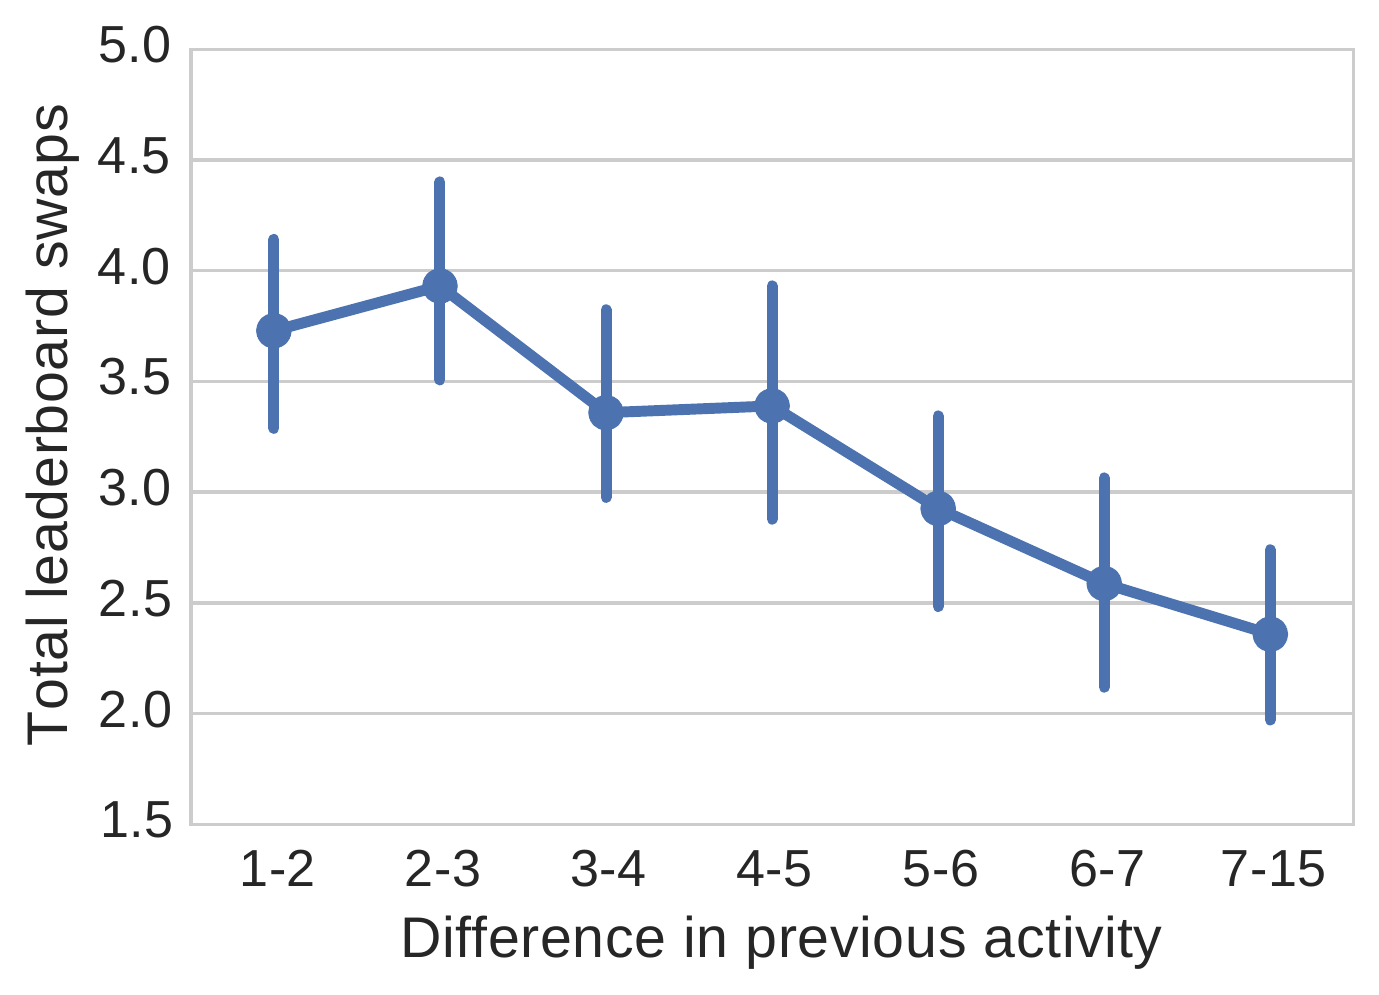}
  %\label{fig:WWW-swaps_vs_max-min}
\end{figure}

\begin{figure}[h!]
\centering
  \centering
  \includegraphics[width=0.5\columnwidth]{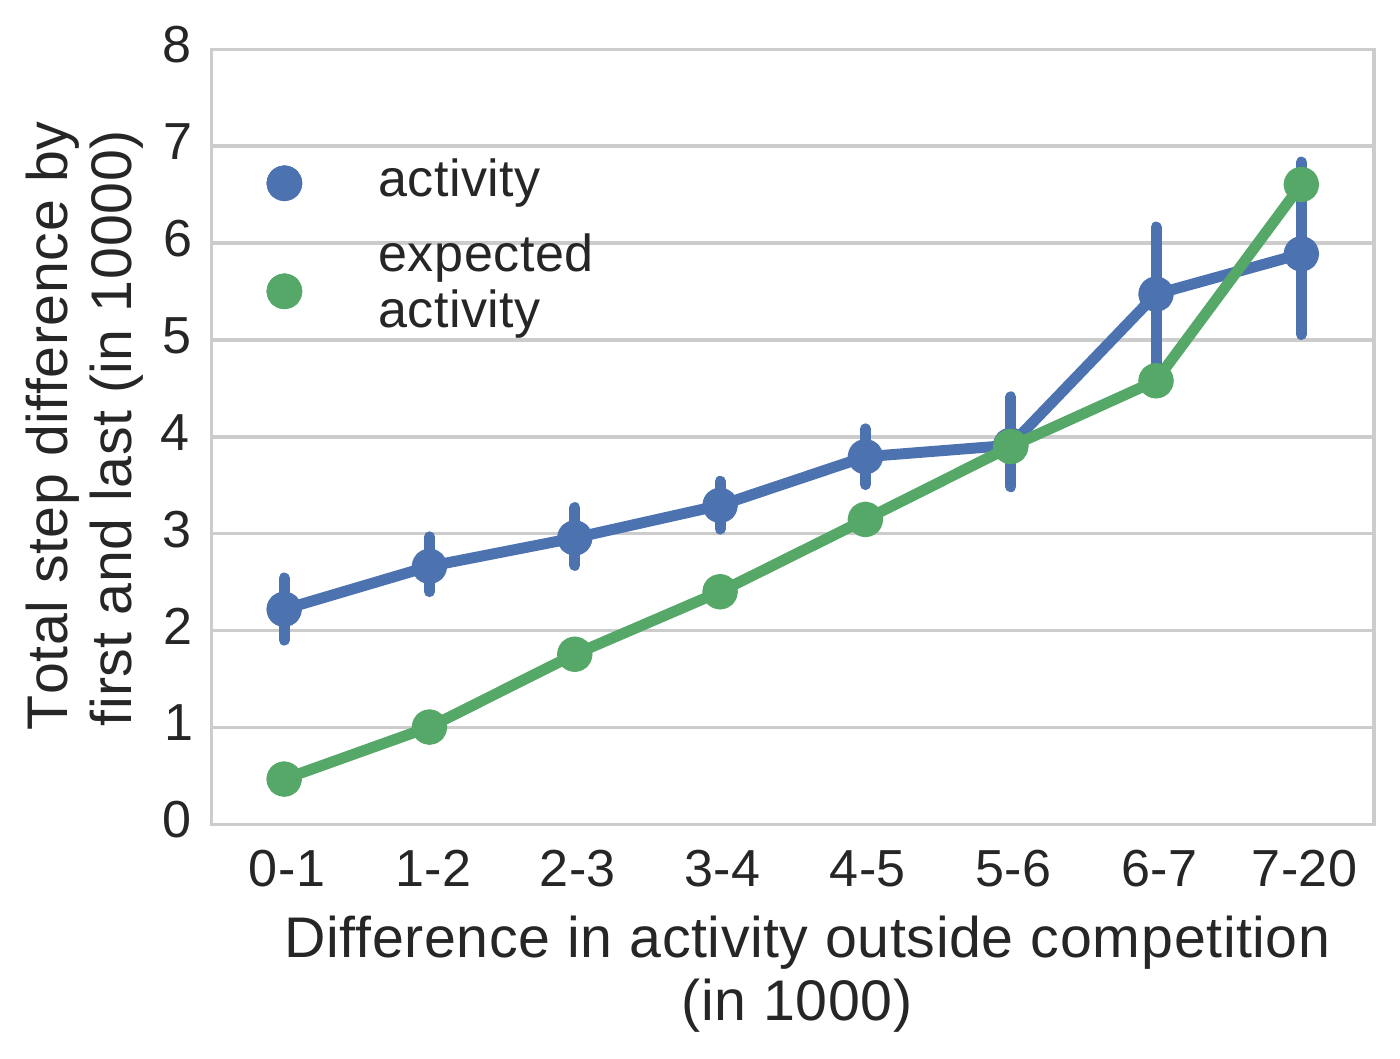}
  \captionof{figure}{}
  %\label{fig:WWW-totalabs_vs_expectedabs}
\end{figure}

\begin{figure}[h!]
\centering
  \centering
  \includegraphics[width=0.5\columnwidth]{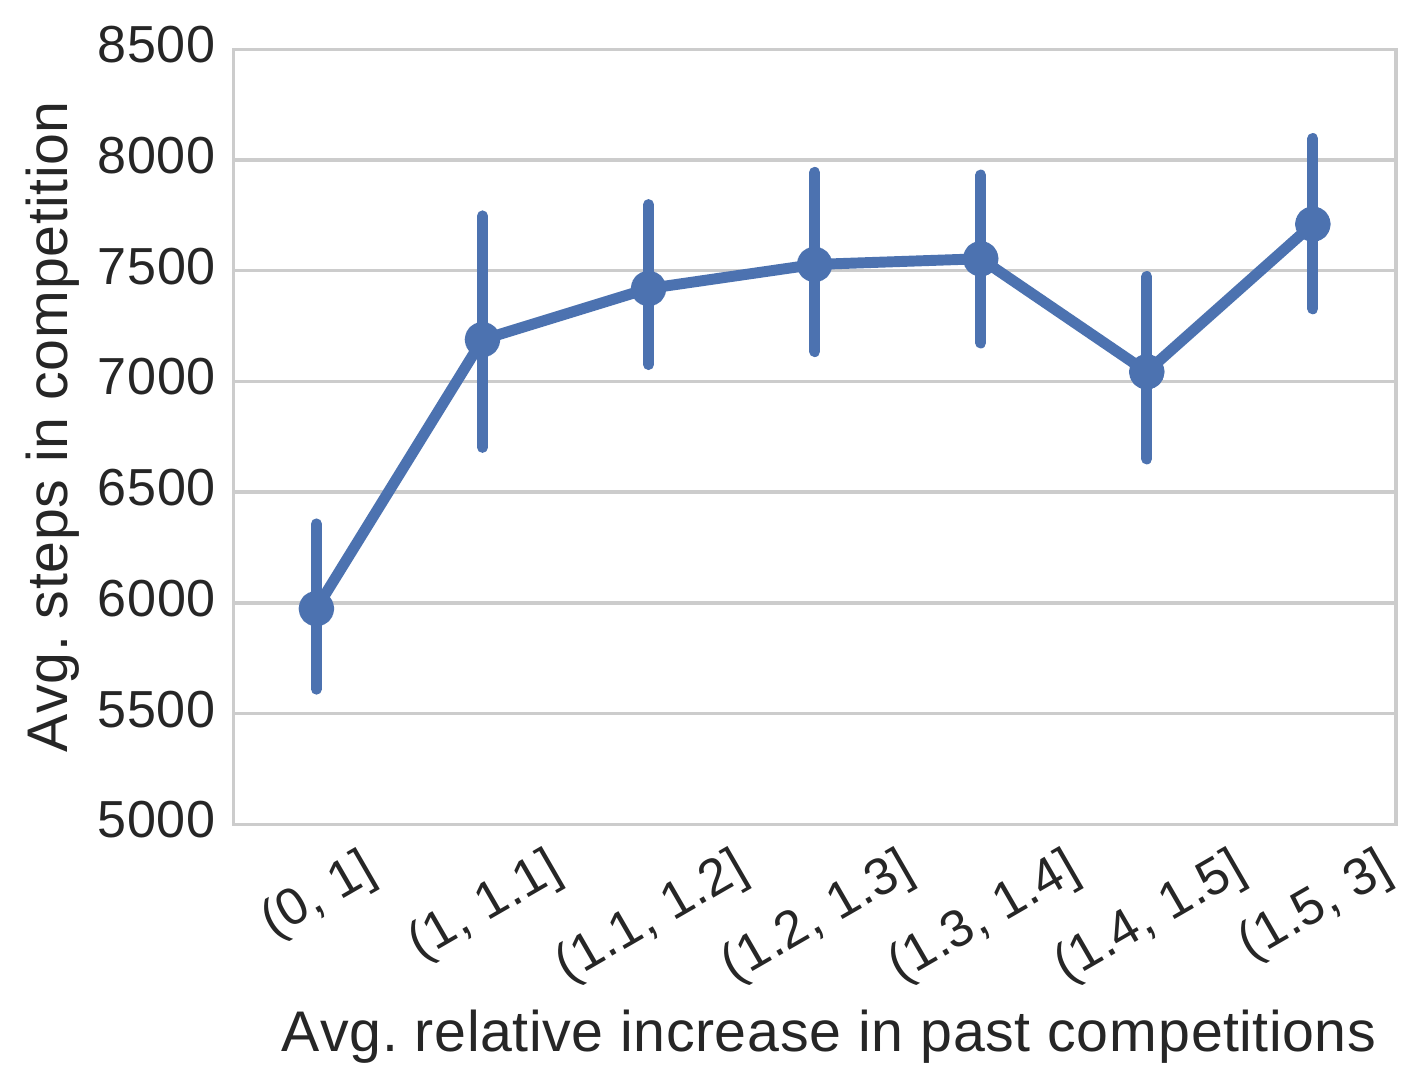}
  \captionof{figure}{}
  %\label{fig:WWW-deltaactivityrel_vs_reldeltamean}
\end{figure}

\begin{figure}[h!]
\centering
  \centering
  \includegraphics[width=0.5\columnwidth]{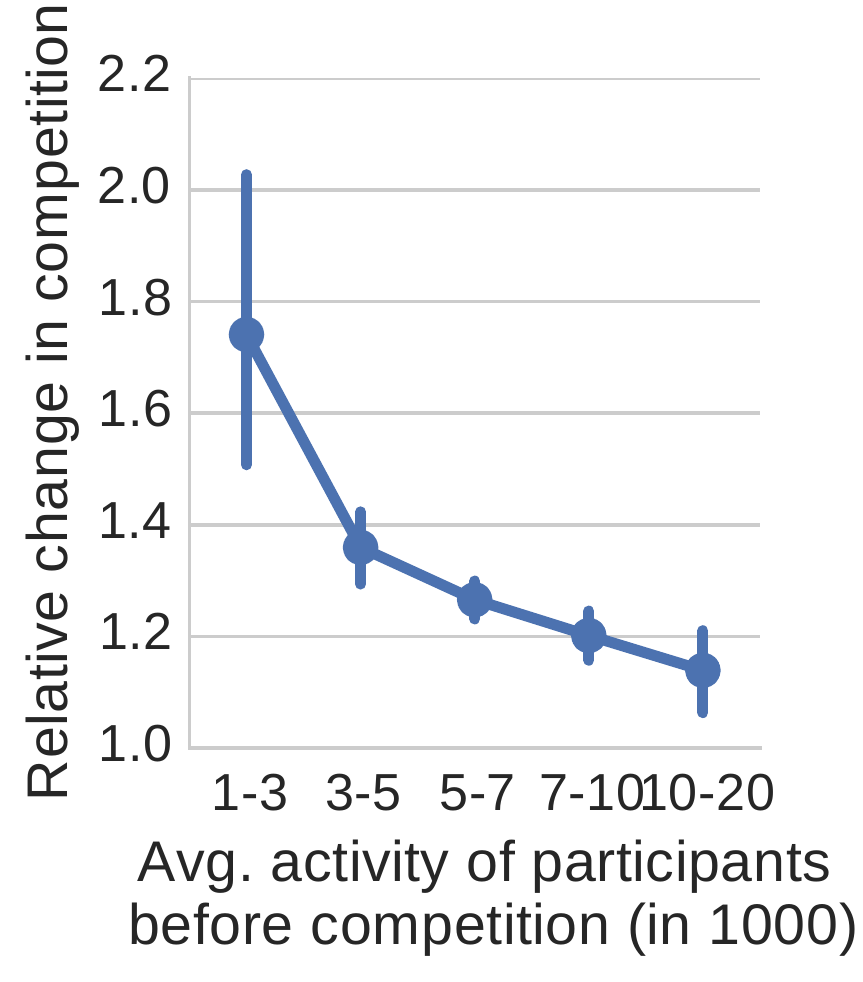}
  \captionof{figure}{}
  %\label{fig:WWW-relchangevsmean}
\end{figure}

\begin{figure}[ht!]
  \centering
  \includegraphics[width=1\columnwidth]{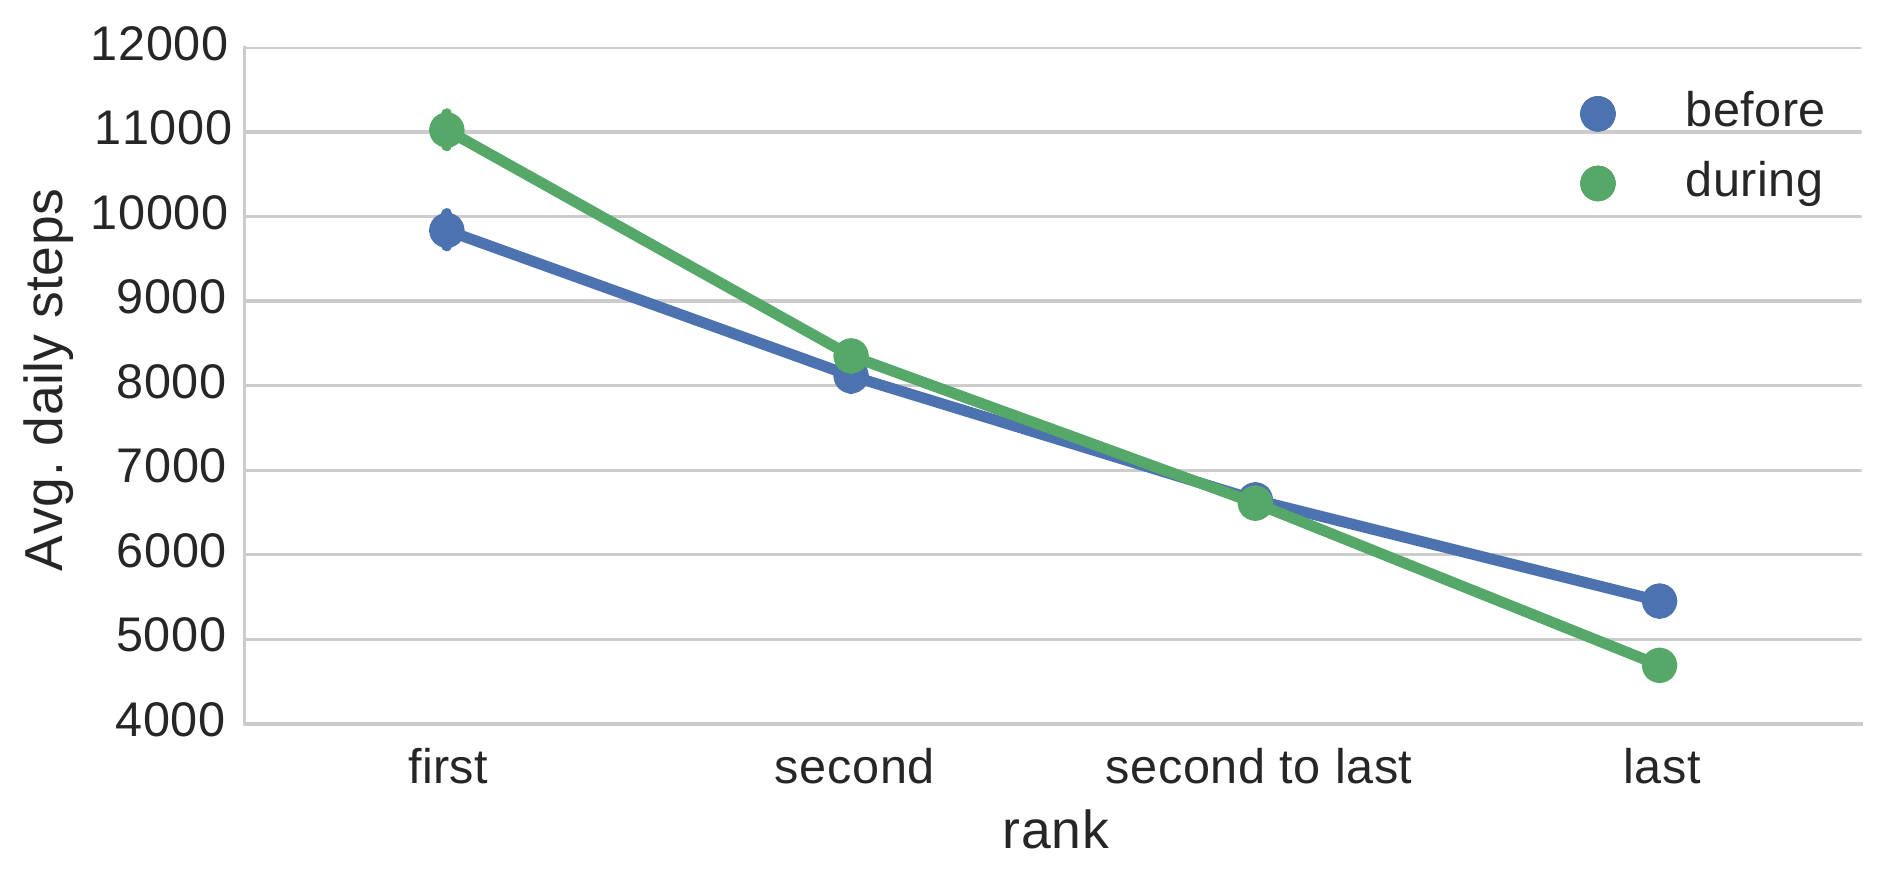}
  \captionof{figure}{Avg. number of steps taken one week before and during a competition for the two top and bottom users.}
  \label{fig:WWW-final-beforeduringafter_lineplot_absolute}
\end{figure}
